# Supplementary material for: EndoVLA-OOV: Language-Conditioned Out-of-View Target Acquisition in Robotic Endoscopy
Source: arXiv:2610.24747 source file (2026-10-17)
Supplement: Supplementary file 1 [file supplement_format.tex]

% Supplementary material follows the manuscript in the same PDF.
\clearpage
\onecolumn
\normalsize
\makeatletter
% Match the supplementary material's original A4, 24 mm margin layout.
\setlength{\paperwidth}{210mm}
\setlength{\paperheight}{297mm}
\pdfpagewidth=\paperwidth
\pdfpageheight=\paperheight
\setlength{\hoffset}{0pt}
\setlength{\voffset}{0pt}
\setlength{\headheight}{14pt}
\setlength{\headsep}{25pt}
\setlength{\footskip}{30pt}
\setlength{\textwidth}{162mm}
\setlength{\textheight}{249mm}
\setlength{\oddsidemargin}{\dimexpr24mm-1in\relax}
\setlength{\evensidemargin}{\oddsidemargin}
\setlength{\topmargin}{\dimexpr24mm-1in-\headheight-\headsep\relax}
\columnwidth=\textwidth
\linewidth=\textwidth
\hsize=\textwidth
\@colht=\textheight
\@colroom=\textheight
\vsize=\textheight
\setlength{\parindent}{0pt}
\setlength{\parskip}{5pt}
\setlength{\abovecaptionskip}{5pt}
\setlength{\belowcaptionskip}{0pt}
\emergencystretch=2em
\raggedbottom
\renewcommand{\section}{\@startsection{section}{1}{\z@}%
 {-3.5ex \@plus -1ex \@minus -.2ex}{1.3ex \@plus .2ex}%
 {\normalfont\Large\bfseries}}
\renewcommand{\subsection}{\@startsection{subsection}{2}{\z@}%
 {-3.25ex \@plus -1ex \@minus -.2ex}{.5ex \@plus .2ex}%
 {\normalfont\large\bfseries}}
\renewcommand{\subsubsection}{\@startsection{subsubsection}{3}{\z@}%
 {-3.25ex \@plus -1ex \@minus -.2ex}{1.5ex \@plus .2ex}%
 {\normalfont\normalsize\bfseries}}
\renewcommand{\@seccntformat}[1]{\csname the#1\endcsname\quad}
\renewcommand{\figurename}{Figure}
\renewcommand{\tablename}{Table}
\renewcommand{\fnum@figure}{\figurename\nobreakspace\thefigure}
\renewcommand{\fnum@table}{\tablename\nobreakspace\thetable}
\long\def\@makecaption#1#2{%
 \vskip\abovecaptionskip
 \begingroup\small\setlength{\parskip}{0pt}\spaceskip=0pt\xspaceskip=0pt
 \sbox\@tempboxa{\textbf{#1:} #2}%
 \ifdim\wd\@tempboxa>\hsize
   \textbf{#1:} #2\par
 \else
   \global\@minipagefalse
   \hb@xt@\hsize{\hfil\box\@tempboxa\hfil}%
 \fi
 \endgroup
 \vskip\belowcaptionskip}
\makeatother
\setcounter{section}{0}
\setcounter{subsection}{0}
\setcounter{figure}{0}
\setcounter{table}{0}
\setcounter{equation}{0}
\renewcommand{\thesection}{S\arabic{section}}
\renewcommand{\thesubsection}{\thesection.\arabic{subsection}}
\renewcommand{\thefigure}{S\arabic{figure}}
\renewcommand{\thetable}{S\arabic{table}}
\renewcommand{\theequation}{S\arabic{equation}}
\renewcommand{\theHsection}{S\arabic{section}}
\renewcommand{\theHsubsection}{\theHsection.\arabic{subsection}}
\renewcommand{\theHfigure}{\thefigure}
\renewcommand{\theHtable}{\thetable}
\renewcommand{\theHequation}{\theequation}
\pagestyle{fancy}
\fancyhf{}
\fancyhead[L]{\small EndoVLA-OOV: Supplementary Information}
\fancyfoot[C]{\thepage}
\renewcommand{\headrulewidth}{0.4pt}
\newcommand{\SIcontentsline}[3]{%
 \noindent\hyperref[#2]{\textbf{#1}\quad #3}\nobreak\dotfill\pageref{#2}\par}
